# Supplementary material for: Identifying the effect of public holidays on daily demand for gas
Source: arXiv:1809.03593 ancillary file (2018-09-12)
Supplement: Supplementary file 1 [file supplMat.pdf]

# Supplementary Materials for Heaps *et al.* (2018)

Sarah E. Heaps
*Newcastle University, Newcastle upon Tyne, UK.*
E-mail: sarah.heaps@ncl.ac.uk
Malcolm Farrow
*Newcastle University, Newcastle upon Tyne, UK.*
Kevin Wilson
*Newcastle University, Newcastle upon Tyne, UK.*

## S1. The composite weather variable (CWV)

For each LDZ, $j = 1, 2$, Figure S1 shows the relationship between log gas demand, $y_{t,j}$, and the mean-centered CWV, $\tilde{w}_{t,j}$, and how this relationship is affected by the raw CWV, $w_{t,j}$. Interpretation of the plot is complicated by the substantially greater density of points in the region where $\tilde{w}_{t,j}$ is close to zero. However, the assumption of a linear relationship, whose slope varies with the raw CWV, appears plausible. Note that any changes in intercept with the raw CWV are likely to be absorbed by the low order harmonics in the smoothed day-of-the week effect $\Gamma_{t,j}$.

## S2. Posterior inference

### *S2.1. Augmented states*

As explained in Section 5 of the main text, the backward smoothing algorithm for quantifying posterior uncertainty in the hidden states $S_t$, $t = 0, \ldots, T$, can be simplified substantially through a reformulation of the model which defines an augmented state $\tilde{S}_t = (S_{t-1}, S_t)'$ for $t = 1, \ldots, T$. The set of 11 permissible values for the augmented state $\tilde{S}_t$ is denoted by $\mathcal{S}_{\tilde{s}}$ and the mapping from $(\mathcal{S}_s \times \mathcal{S}_s)$ to $\mathcal{S}_{\tilde{s}}$ is given in Table S1. The representation of the transition matrix for the new hidden process in terms of the original transition probabilities is indicated in Table S2.

The forward filtering algorithm for this reformulation of the NHMM is given in Section S2.2 whilst the backward smoothing algorithm is provided in Section S2.3.

### *S2.2. Forward filtering algorithm to compute the observed data likelihood*

Table S1 implies a mapping from the augmented state $\tilde{S}_t \in \mathcal{S}_{\tilde{s}}$ to its original parts $S_{t-1} \in \mathcal{S}_s$ and $S_t \in \mathcal{S}_s$. Denote these mappings by $f : \mathcal{S}_{\tilde{s}} \to \mathcal{S}_s$ and $g : \mathcal{S}_{\tilde{s}} \to \mathcal{S}_s$, respectively. For example, $f(4) = 2$ and $g(4) = 3$. For each $\ell \in \mathcal{S}_{\tilde{s}}$, the set $\mathcal{P}_\ell = \{k \in \mathcal{S}_{\tilde{s}} : f(k) = g(\ell)\}$ is defined as the collection of augmented states from which $\ell$ can be reached in a single transition; see Table S1. Using this notation, the forward filter can be expressed as follows.

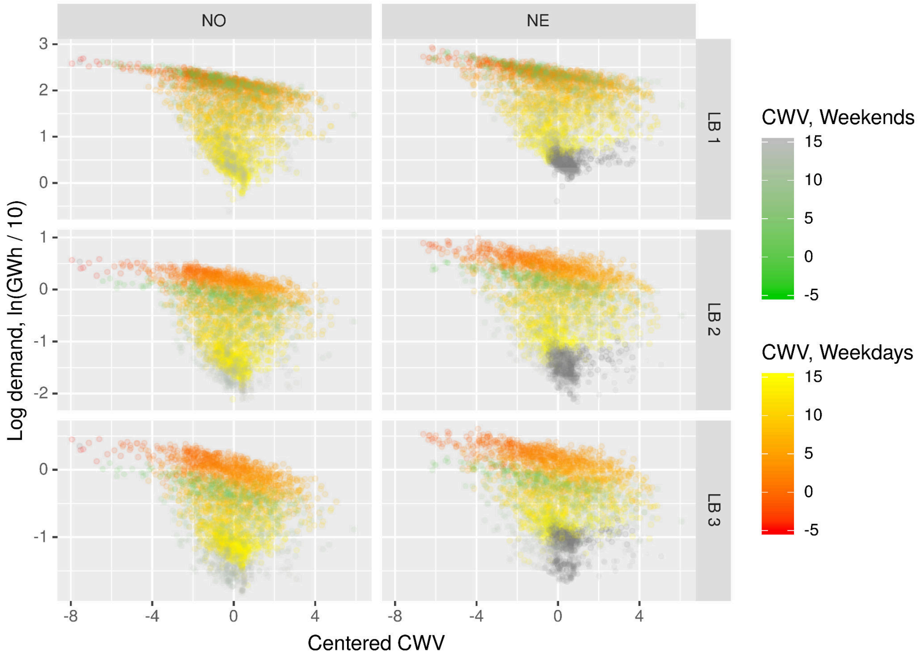


**Fig. S1.** Scatter plot of the natural logarithm of gas demand against the mean-centered composite weather variable for both LDZs in each NDM load band. Two continuous colour gradients indicate the effect of the raw composite weather variable, stratified by the type of day.

1. Initialise the forward recursion at time $t = 1$:

$$\begin{aligned}\Pr(\tilde{S}_1 = k, \boldsymbol{y}_1 | \Pi, \Lambda, \boldsymbol{n}, \boldsymbol{p}, \boldsymbol{r}, \boldsymbol{w}) &= p(\boldsymbol{y}_1 | \tilde{S}_1 = k, \Pi, \boldsymbol{w}_1, n_1, p_1, r_1) \Pr(\tilde{S}_1 = k | \Lambda, \boldsymbol{n}_{0:1}, \boldsymbol{p}_{0:1}) \\ &= p(\boldsymbol{y}_1 | S_1 = g(k), \Pi, \boldsymbol{w}_1, n_1, p_1, r_1) \\ &\qquad \times \ell_{f(k)}(n_0, p_0) \lambda_{f(k), g(k)}(n_1, p_1)\end{aligned}$$

for $k \in \mathcal{S}_{\tilde{s}}$, where the density $p(\boldsymbol{y}_1 | S_1 = s_1, \Pi, \boldsymbol{w}_1, n_1, p_1, r_1)$ is defined through (6).

2. For $t = 2, \ldots, T$ in a forward recursion:

$$\begin{aligned}&\Pr(\tilde{S}_t = k, \boldsymbol{y}_{1:t} | \Pi, \Lambda, \boldsymbol{n}, \boldsymbol{p}, \boldsymbol{r}, \boldsymbol{w}) \\ &\quad = p(\boldsymbol{y}_t | \boldsymbol{y}_{t-1}, \tilde{S}_t = k, \Pi, \Lambda, n_t, p_t, r_t, \boldsymbol{w}_t) \\ &\qquad \times \sum_{j \in \mathcal{P}_k} \Pr(\tilde{S}_t = k | \tilde{S}_{t-1} = j, \Lambda, n_t, p_t) \Pr(\tilde{S}_{t-1} = j, \boldsymbol{y}_{1:t-1} | \Pi, \Lambda, \boldsymbol{n}, \boldsymbol{p}, \boldsymbol{r}, \boldsymbol{w}) \\ &\quad = p(\boldsymbol{y}_t | \boldsymbol{y}_{t-1}, S_{t-1} = f(k), S_t = g(k), \Pi, n_t, p_t, r_t, \boldsymbol{w}_t) \\ &\qquad \times \lambda_{f(k), g(k)}(n_t, p_t) \sum_{j \in \mathcal{P}_k} \Pr(\tilde{S}_{t-1} = j, \boldsymbol{y}_{1:t-1} | \Pi, \Lambda, \boldsymbol{n}, \boldsymbol{p}, \boldsymbol{r}, \boldsymbol{w})\end{aligned}$$

for $k \in \mathcal{S}_{\tilde{s}}$, where the density $p(\boldsymbol{y}_t | \boldsymbol{y}_{t-1}, S_{t-1} = j, S_t = k, \Pi, n_t, p_t, r_t, \boldsymbol{w}_t)$ is defined through (5).

**Table S1.** The mapping from the original states $(S_{t-1}, S_t) \in (\mathcal{S}_s \times \mathcal{S}_s)$ to the augmented states $\tilde{S}_t \in \mathcal{S}_{\tilde{s}}$. Also shown are the sets (i) $\mathcal{P}_\ell = \{k \in \mathcal{S}_{\tilde{s}} : f(k) = g(\ell)\}$ of augmented states from which state $\ell$ can be reached in a single transition and (ii) $\mathcal{N}_\ell = \{k \in \mathcal{S}_{\tilde{s}} : g(k) = f(\ell)\}$ of augmented states that can be reached from state $\ell$ in a single transition.

| $(S_{t-1}, S_t)$ | $\tilde{S}_t$ | $\mathcal{P}_{\tilde{S}_t}$ | $\mathcal{N}_{\tilde{S}_t}$ |
|---|---|---|---|
| (1,1) | 1 | 1, 9 | 1, 2 |
| (1,2) | 2 | 1, 9 | 3, 4, 5 |
| (2,2) | 3 | 2, 3, 6, 10 | 3, 4, 5 |
| (2,3) | 4 | 2, 3, 6, 10 | 6, 7, 8 |
| (2,4) | 5 | 2, 3, 6, 10 | 9, 10, 11 |
| (3,2) | 6 | 4, 7 | 3, 4, 5 |
| (3,3) | 7 | 4, 7 | 6, 7, 8 |
| (3,4) | 8 | 4, 7 | 9, 10, 11 |
| (4,1) | 9 | 5, 8, 11 | 1, 2 |
| (4,2) | 10 | 5, 8, 11 | 3, 4, 5 |
| (4,4) | 11 | 5, 8, 11 | 9, 10, 11 |

3. Compute the observed data likelihood:

$$p(\boldsymbol{y}|\Pi, \Lambda, \boldsymbol{n}, \boldsymbol{p}, \boldsymbol{r}, \boldsymbol{w}) = \sum_{k \in \mathcal{S}_{\tilde{s}}} \Pr(\tilde{S}_T = k, \boldsymbol{y}_{1:T}|\Pi, \Lambda, \boldsymbol{n}, \boldsymbol{p}, \boldsymbol{r}, \boldsymbol{w}).$$

### *S2.3. Backward algorithm to compute the smoothed probabilities*

For each $\ell \in \mathcal{S}_{\tilde{s}}$, the set $\mathcal{N}_\ell = \{k \in \mathcal{S}_{\tilde{s}} : g(k) = f(\ell)\}$ is defined as the collection of augmented states that can be reached from $\ell$ in a single transition; see Table S1. Using this notation, the backward smoothing algorithm can be expressed as follows.

1. Use the forward filtering algorithm described in Section S2.2 to compute the probabilities $\Pr(\tilde{S}_t = k, \boldsymbol{y}_{1:t}|\Pi, \Lambda, \boldsymbol{n}, \boldsymbol{p}, \boldsymbol{r}, \boldsymbol{w})$, $k \in \mathcal{S}_{\tilde{s}}$, for $t = 1, 2, \ldots, T$, and the observed data likelihood $p(\boldsymbol{y}|\Pi, \Lambda, \boldsymbol{n}, \boldsymbol{p}, \boldsymbol{r}, \boldsymbol{w})$.

2. Initialise the backward recursion at time $t = T$ by computing:

$$\Pr(\tilde{S}_T = k|\boldsymbol{y}, \Pi, \Lambda, \boldsymbol{n}, \boldsymbol{p}, \boldsymbol{r}, \boldsymbol{w}) = \frac{\Pr(\tilde{S}_T = k, \boldsymbol{y}_{1:T}|\Pi, \Lambda, \boldsymbol{n}, \boldsymbol{p}, \boldsymbol{r}, \boldsymbol{w})}{p(\boldsymbol{y}|\Pi, \Lambda, \boldsymbol{n}, \boldsymbol{p}, \boldsymbol{r}, \boldsymbol{w})}$$

   for $k \in \mathcal{S}_{\tilde{s}}$.

**Table S2.** The transition matrix for the augmented state process on a day which is (a) not a public holiday and (b) a public holiday.

(a) Not public holiday.

| $\tilde{S}_{t-1}$ | $\tilde{S}_t$ | | | | | | | | | | |
|---|---|---|---|---|---|---|---|---|---|---|---|
| | 1 | 2 | 3 | 4 | 5 | 6 | 7 | 8 | 9 | 10 | 11 |
| 1 | 1 | 0 | 0 | 0 | 0 | 0 | 0 | 0 | 0 | 0 | 0 |
| 2 | 0 | 0 | 0 | $\lambda_{2,3}(\cdot)$ | $\lambda_{2,4}(\cdot)$ | 0 | 0 | 0 | 0 | 0 | 0 |
| 3 | 0 | 0 | 0 | $\lambda_{2,3}(\cdot)$ | $\lambda_{2,4}(\cdot)$ | 0 | 0 | 0 | 0 | 0 | 0 |
| 4 | 0 | 0 | 0 | 0 | 0 | 0 | $\lambda_{3,3}(\cdot)$ | $\lambda_{3,4}(\cdot)$ | 0 | 0 | 0 |
| 5 | 0 | 0 | 0 | 0 | 0 | 0 | 0 | 0 | $\lambda_{4,1}(\cdot)$ | 0 | $\lambda_{4,4}(\cdot)$ |
| 6 | 0 | 0 | 0 | $\lambda_{2,3}(\cdot)$ | $\lambda_{2,4}(\cdot)$ | 0 | 0 | 0 | 0 | 0 | 0 |
| 7 | 0 | 0 | 0 | 0 | 0 | 0 | $\lambda_{3,3}(\cdot)$ | $\lambda_{3,4}(\cdot)$ | 0 | 0 | 0 |
| 8 | 0 | 0 | 0 | 0 | 0 | 0 | 0 | 0 | $\lambda_{4,1}(\cdot)$ | 0 | $\lambda_{4,4}(\cdot)$ |
| 9 | 1 | 0 | 0 | 0 | 0 | 0 | 0 | 0 | 0 | 0 | 0 |
| 10 | 0 | 0 | 0 | $\lambda_{2,3}(\cdot)$ | $\lambda_{2,4}(\cdot)$ | 0 | 0 | 0 | 0 | 0 | 0 |
| 11 | 0 | 0 | 0 | 0 | 0 | 0 | 0 | 0 | $\lambda_{4,1}(\cdot)$ | 0 | $\lambda_{4,4}(\cdot)$ |

(b) Public holiday.

| $\tilde{S}_{t-1}$ | $\tilde{S}_t$ | | | | | | | | | | |
|---|---|---|---|---|---|---|---|---|---|---|---|
| | 1 | 2 | 3 | 4 | 5 | 6 | 7 | 8 | 9 | 10 | 11 |
| 1 | 0 | 1 | 0 | 0 | 0 | 0 | 0 | 0 | 0 | 0 | 0 |
| 2 | 0 | 0 | 1 | 0 | 0 | 0 | 0 | 0 | 0 | 0 | 0 |
| 3 | 0 | 0 | 1 | 0 | 0 | 0 | 0 | 0 | 0 | 0 | 0 |
| 4 | 0 | 0 | 0 | 0 | 0 | 1 | 0 | 0 | 0 | 0 | 0 |
| 5 | 0 | 0 | 0 | 0 | 0 | 0 | 0 | 0 | 0 | 1 | 0 |
| 6 | 0 | 0 | 1 | 0 | 0 | 0 | 0 | 0 | 0 | 0 | 0 |
| 7 | 0 | 0 | 0 | 0 | 0 | 1 | 0 | 0 | 0 | 0 | 0 |
| 8 | 0 | 0 | 0 | 0 | 0 | 0 | 0 | 0 | 0 | 1 | 0 |
| 9 | 0 | 1 | 0 | 0 | 0 | 0 | 0 | 0 | 0 | 0 | 0 |
| 10 | 0 | 0 | 1 | 0 | 0 | 0 | 0 | 0 | 0 | 0 | 0 |
| 11 | 0 | 0 | 0 | 0 | 0 | 0 | 0 | 0 | 0 | 1 | 0 |

3. For $t = T-1, T-2, \ldots, 1$ in a backward recursion compute:

$$\begin{aligned}
&\Pr(\tilde{S}_t = k|\boldsymbol{y}, \Pi, \Lambda, \boldsymbol{n}, \boldsymbol{p}, \boldsymbol{r}, \boldsymbol{w}) \\
&\quad = \Pr(\tilde{S}_t = k, \boldsymbol{y}_{1:t}|\Pi, \Lambda, \boldsymbol{n}, \boldsymbol{p}, \boldsymbol{r}, \boldsymbol{w}) \\
&\quad\quad \times \sum_{\ell \in \mathcal{N}_k} \frac{\Pr(\tilde{S}_{t+1} = \ell|\tilde{S}_t = k, \Lambda, n_{t+1}, p_{t+1}) \Pr(\tilde{S}_{t+1} = \ell|\boldsymbol{y}, \Pi, \Lambda, \boldsymbol{n}, \boldsymbol{p}, \boldsymbol{r}, \boldsymbol{w})}{\sum_{j \in \mathcal{P}_\ell} \Pr(\tilde{S}_{t+1} = \ell|\tilde{S}_t = j, \Lambda, n_{t+1}, p_{t+1}) \Pr(\tilde{S}_t = j, \boldsymbol{y}_{1:t}|\Pi, \Lambda, \boldsymbol{n}, \boldsymbol{p}, \boldsymbol{r}, \boldsymbol{w})} \\
&\quad = \Pr(\tilde{S}_t = k, \boldsymbol{y}_{1:t}|\Pi, \Lambda, \boldsymbol{n}, \boldsymbol{p}, \boldsymbol{r}, \boldsymbol{w}) \\
&\quad\quad \times \sum_{\ell \in \mathcal{N}_k} \frac{\lambda_{g(\ell), f(\ell)}(n_{t+1}, p_{t+1}) \Pr(\tilde{S}_{t+1} = \ell|\boldsymbol{y}, \Pi, \Lambda, \boldsymbol{n}, \boldsymbol{p}, \boldsymbol{r}, \boldsymbol{w})}{\sum_{j \in \mathcal{P}_\ell} \lambda_{g(\ell), f(\ell)}(n_{t+1}, p_{t+1}) \Pr(\tilde{S}_t = j, \boldsymbol{y}_{1:t}|\Pi, \Lambda, \boldsymbol{n}, \boldsymbol{p}, \boldsymbol{r}, \boldsymbol{w})} \\
&\quad = \Pr(\tilde{S}_t = k, \boldsymbol{y}_{1:t}|\Pi, \Lambda, \boldsymbol{n}, \boldsymbol{p}, \boldsymbol{r}, \boldsymbol{w}) \sum_{\ell \in \mathcal{N}_k} \frac{\Pr(\tilde{S}_{t+1} = \ell|\boldsymbol{y}, \Pi, \Lambda, \boldsymbol{n}, \boldsymbol{p}, \boldsymbol{r}, \boldsymbol{w})}{\sum_{j \in \mathcal{P}_\ell} \Pr(\tilde{S}_t = j, \boldsymbol{y}_{1:t}|\Pi, \Lambda, \boldsymbol{n}, \boldsymbol{p}, \boldsymbol{r}, \boldsymbol{w})}
\end{aligned}$$

   for $k \in \mathcal{S}_{\tilde{s}}$.

4. For $t = 0$ marginalise over $S_1$ in the smoothed probability for $\tilde{S}_1 = (S_0, S_1)$ to compute:

$$\Pr(S_0 = k|\boldsymbol{y}, \Pi, \Lambda, \boldsymbol{n}, \boldsymbol{p}, \boldsymbol{r}, \boldsymbol{w}) = \sum_{\ell : f(\ell) = k} \Pr(\tilde{S}_1 = \ell|\boldsymbol{y}, \Pi, \Lambda, \boldsymbol{n}, \boldsymbol{p}, \boldsymbol{r}, \boldsymbol{w})$$

   for $k \in \mathcal{S}_s$. Similarly, for $t = 1, \ldots, T$ marginalise over $S_{t-1}$ in the smoothed probability for $\tilde{S}_t = (S_{t-1}, S_t)$ to compute:

$$Pr(S_t = k|\boldsymbol{y}, \Pi, \Lambda, \boldsymbol{n}, \boldsymbol{p}, \boldsymbol{r}, \boldsymbol{w}) = \sum_{\ell : g(\ell) = k} \Pr(\tilde{S}_t = \ell|\boldsymbol{y}, \Pi, \Lambda, \boldsymbol{n}, \boldsymbol{p}, \boldsymbol{r}, \boldsymbol{w})$$

   for $k \in \mathcal{S}_s$.

## S3. Prior specification

The prior distribution for the model parameters was outlined in Section 4 of the main text. Section 6.1 then provided comments on its use in the NGN application. Further details are given below.

### *S3.1. Parameters of the conditional demand model*

The structure of our prior for the parameters $\Pi$ in the conditional model for gas demand given the states was outlined in Section 4.2 in the main text. The moments in this prior were fixed through the following prior specification.

In the prior for the intercept, and the weather, seasonal and calendar effects in the time-varying mean $\boldsymbol{\mu}_t$ we chose the marginal prior variances

$$v_\alpha = v_{\zeta,1} = v_{\zeta,2} = v_\delta = v_{\gamma,1} = v_{\gamma,2} = 100, \qquad v_{\gamma,3} = v_{\gamma,4} = 1, \qquad v_{\gamma,5} = v_{\gamma,6} = 0.01$$

and the correlations between sites

$$r_\alpha = r_{\zeta,1} = r_{\zeta,2} = r_\delta = r_\gamma = 0.85.$$

We chose marginal prior means of $m_\alpha = 0$ for the intercept and $m_{\zeta,1} = m_{\zeta,2} = 0$ for the CWV coefficients.

In the prior for the public holiday effects, we set the correlation between sites at $r_\beta = 0.85$ and adopted a compound symmetric structure for the prior variance matrix with

$$V_\beta = (d_\beta - c_\beta)I_3 + c_\beta J_3$$

where $J_m$ is an $(m \times m)$ matrix of 1s. Here we chose $d_\beta = 1$ and $c_\beta = 0.95$ for NDM load band 1, for which we anticipated a smaller effect, and $d_\beta = 10$ and $c_\beta = 9.5$ in NDM load bands 2 and 3.

For the logit of the decay parameters in our asymmetric hierarchical prior, we chose the mean, variance and correlation parameters to be

$$m_{\tilde{\rho}} = 0, \qquad v_{\tilde{\rho}} = 0.25, \qquad r_{\tilde{\rho},1} = 0.85, \qquad r_{\tilde{\rho},2} = 0.85$$

so that $\mathrm{Cor}(\tilde{\rho}_{\beta,1}, \tilde{\rho}_{\beta,2}) = 0.85$ but $\mathrm{Cor}(\tilde{\rho}_{\beta,j}, \tilde{\rho}_\theta) = 0.78$ for $j = 1, 2$.

Finally, for the parameters in the time-varying precision matrix $\Omega_t$, the priors for the intercept, public holiday effect and seasonal effects had variances

$$v_{\eta,i} = v_{\kappa,i,1} = v_{\kappa,i,2} = 100, \qquad v_{\theta,i} = v_{\kappa,i,3} = \ldots = v_{\kappa,i,10} = 1, \qquad v_{\kappa,i,11} = v_{\kappa,i,12} = 0.01$$

for $i = 1, 2, 3$, along with prior means of $m_{\eta,i} = 0$, $i = 1, 2, 3$, for each intercept. For the parameters in prior for the reparameterised autoregressive coefficient matrix, we chose $a_{\xi,i} = b_{\xi,i} = 1$ for $i = 1, 2$.

### *S3.2. Transition probabilities*

The structure of our prior for the parameters $\Lambda$ in the model for the hidden states was outlined in Section 4.1 in the main text. The means and variances in the independent normal components were fixed through the following prior specification.

$$\begin{aligned} \boldsymbol{m}_{2,3,1:2} &= (0, 0.25)', & \boldsymbol{v}_{2,3,1:2} &= (1, 1)', \\ \boldsymbol{m}_{3,4,1:3} &= (-0.5, 0, -1)', & \boldsymbol{v}_{3,4,1:3} &= (1, 1, 1)', \\ \boldsymbol{m}_{4,1,1:2} &= (-1, -13)', & \boldsymbol{v}_{4,1,1:2} &= (0.5, 4)'. \end{aligned}$$

This yielded the pointwise prior mode for the state sequence depicted in Figure S2.

## S4. Posterior inference

### *S4.1. State inference*

For load bands 1 and 2, Figures S3 and S4 show the posterior distribution for the states $S_t$ in a representative year (2015), with the prior distribution overlaid. The corresponding plot for load band 3 was given in Figure 7 of the main text.

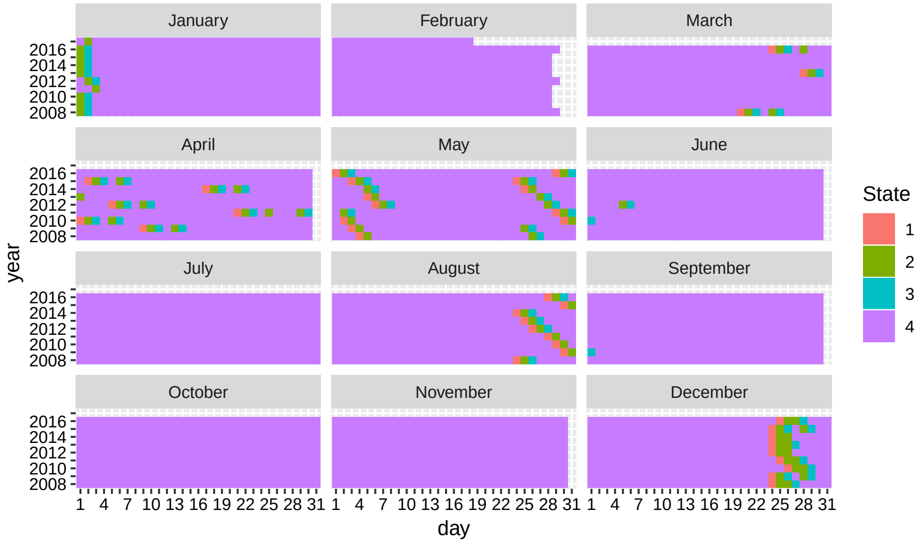


**Fig. S2.** Pointwise prior mode for the state sequence $S_t$.

### *S4.2. Posterior predictive inference*

Section 6.3.3 of the main text describes a simplified version of our four state NHMM which ignores the proximity effect and omits the pre- and post-holiday states (states 1 and 3). That is, under the simplified two-state model, each day is classified either as a public holiday (state 2) or not (state 4). For load band 3, for all the days during the observation period which were ten days away from a public holiday, Figure S5 compares the posterior predictive distribution for log gas demand under the two models to the values that were observed. The corresponding plots for days which were public holidays and one day from a public holiday were given in Figures 8 and 9 of the main text where comments were provided. An analogous set of plots for load band 2 is given in Figures S6–S8 below.

In terms of the proportion of observations lying outside the central 95% of their posterior predictive distribution, Table S3 contains a summary across all load bands.

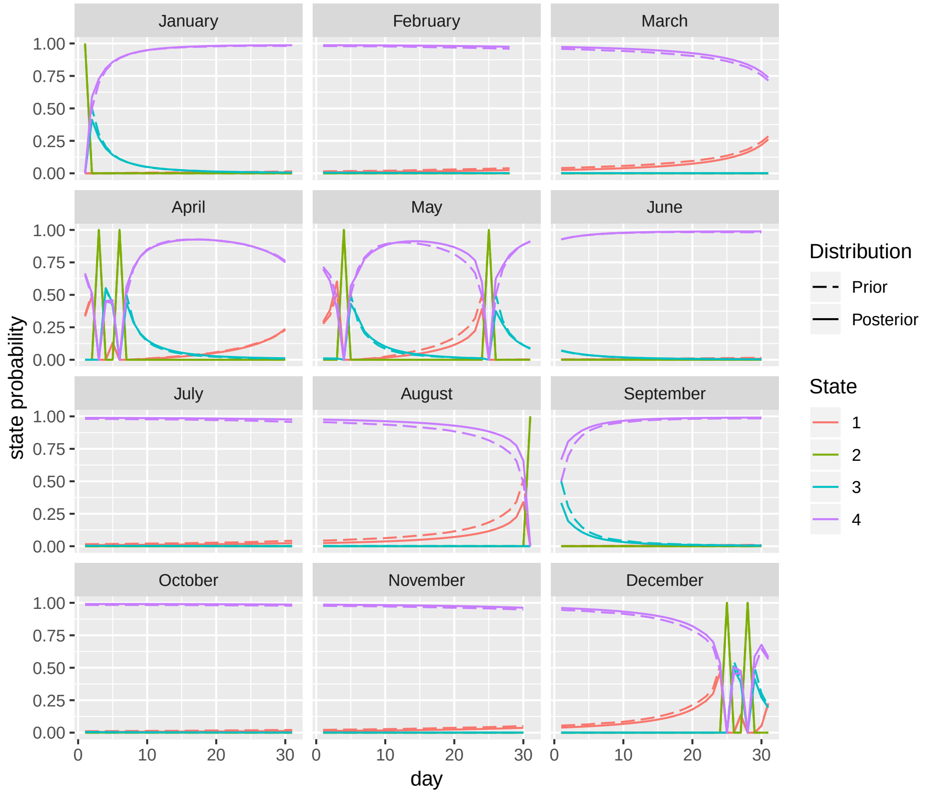


**Fig. S3.** Prior and posterior for the state sequence $S_t$ for load band 1 in an illustrative year (2015).

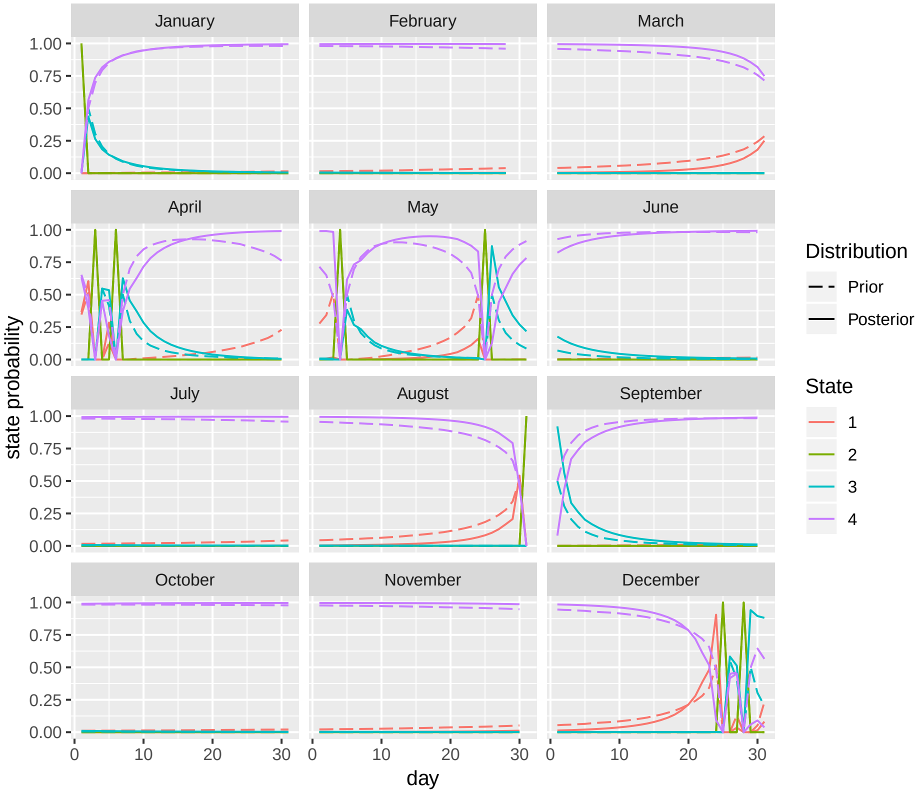


**Fig. S4.** Prior and posterior for the state sequence $S_t$ for load band 2 in an illustrative year (2015).

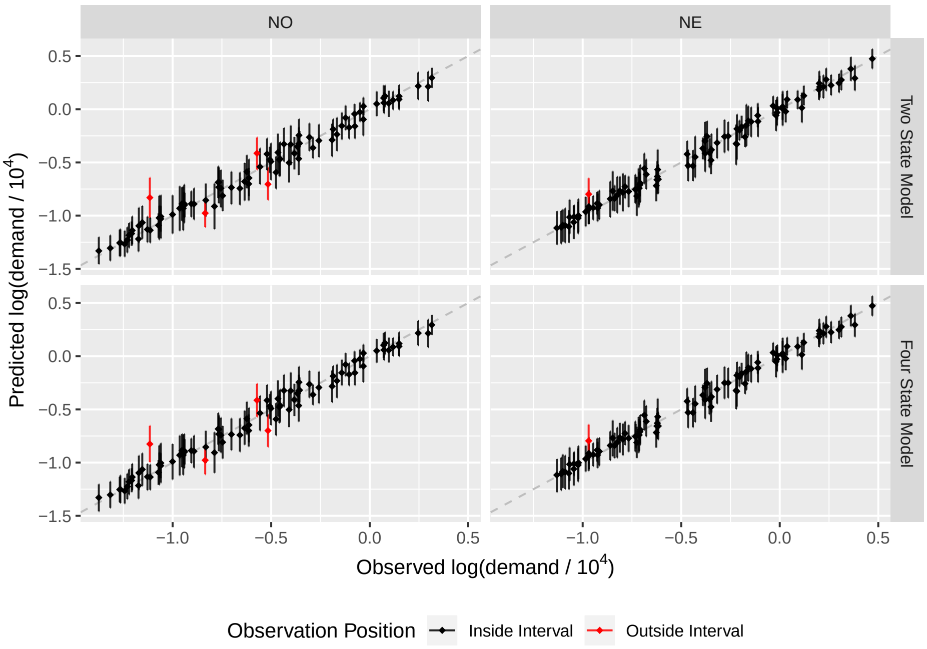


**Fig. S5.** For load band 3 and each LDZ, posterior predictive means versus observed log gas demand for each day in the observation period which was ten days from a public holiday. Vertical bars extend to the 2.5% and 97.5% points in the posterior predictive distributions. Colours indicate whether the observation lay inside or outside the central 95% of the posterior predictive distribution. Upper panels are based on the simple two-state model, lower panels on the four-state NHMM.

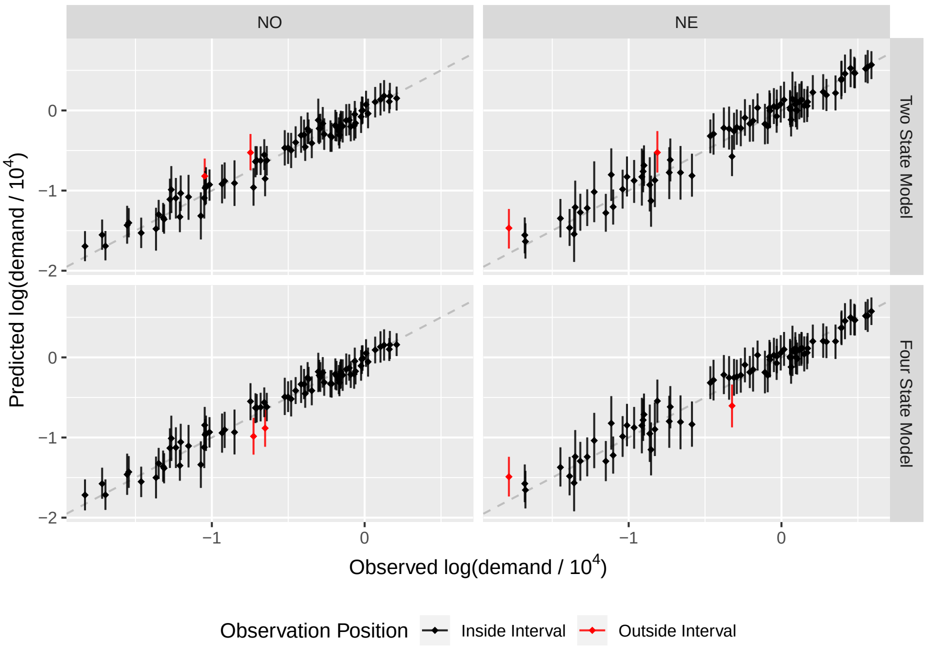


**Fig. S6.** For load band 2 and each LDZ, posterior predictive means versus observed log gas demand for each public holiday in the observation period. Vertical bars extend to the 2.5% and 97.5% points in the posterior predictive distributions. Colours indicate whether the observation lay inside or outside the central 95% of the posterior predictive distribution. Upper panels are based on the simple two-state model, lower panels on the four-state NHMM.

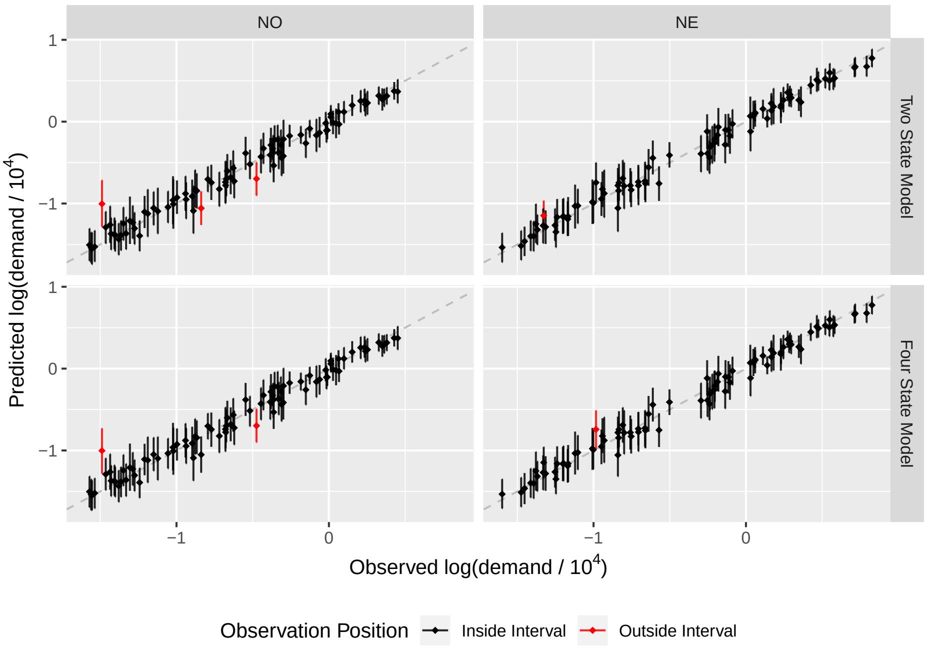


**Fig. S7.** For load band 2 and each LDZ, posterior predictive means versus observed log gas demand for each day in the observation period which was ten days from a public holiday. Vertical bars extend to the 2.5% and 97.5% points in the posterior predictive distributions. Colours indicate whether the observation lay inside or outside the central 95% of the posterior predictive distribution. Upper panels are based on the simple two-state model, lower panels on the four-state NHMM.

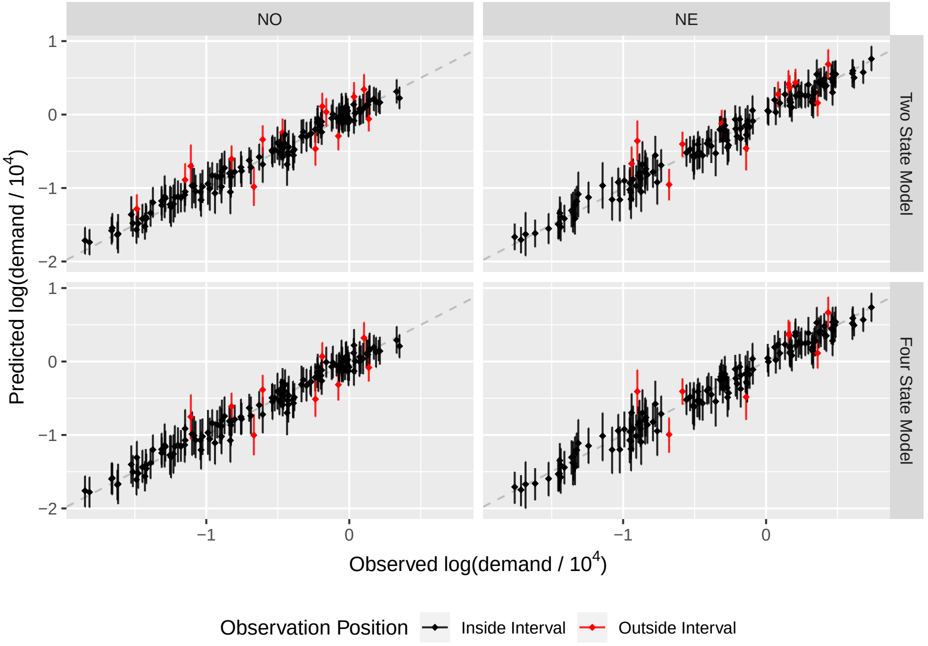


**Fig. S8.** For load band 2 and each LDZ, posterior predictive means versus observed log gas demand for each day in the observation period which was one day from a public holiday. Vertical bars extend to the 2.5% and 97.5% points in the posterior predictive distributions. Colours indicate whether the observation lay inside or outside the central 95% of the posterior predictive distribution. Upper panels are based on the simple two-state model, lower panels on the four-state NHMM.

**Table S3.** Proportion of observations lying outside the central 95% of their posterior predictive distribution under the simplified two state model (2 St.) and the four state NHMM (4 St.). Results are shown for both the NO and NE LDZ and for each load band (LB).

| Gap | NO | | | | | | NE | | | | | |
|---|---|---|---|---|---|---|---|---|---|---|---|---|
| | LB 1 | | LB 2 | | LB 3 | | LB 1 | | LB 2 | | LB 3 | |
| | 2 St. | 4 St. | 2 St. | 4 St. | 2 St. | 4 St. | 2 St. | 4 St. | 2 St. | 4 St. | 2 St. | 4 St. |
| 0 | 4.00 | 5.33 | 2.67 | 2.67 | 5.33 | 2.67 | 5.33 | 6.67 | 2.67 | 2.67 | 5.33 | 4.00 |
| 1 | 5.93 | 4.44 | 10.37 | 6.67 | 9.63 | 5.19 | 5.19 | 4.44 | 8.89 | 5.93 | 10.37 | 4.44 |
| 2 | 2.78 | 3.70 | 6.48 | 6.48 | 5.56 | 5.56 | 9.26 | 7.41 | 7.41 | 7.41 | 8.33 | 5.56 |
| 3 | 9.18 | 10.20 | 10.20 | 8.16 | 8.16 | 8.16 | 3.06 | 2.04 | 5.10 | 4.08 | 7.14 | 7.14 |
| 4 | 5.56 | 6.67 | 5.56 | 6.67 | 6.67 | 7.78 | 4.44 | 4.44 | 7.78 | 7.78 | 8.89 | 7.78 |
| 5 | 2.25 | 2.25 | 6.74 | 6.74 | 2.25 | 2.25 | 2.25 | 3.37 | 3.37 | 3.37 | 2.25 | 2.25 |
| ⋮ | ⋮ | ⋮ | ⋮ | ⋮ | ⋮ | ⋮ | ⋮ | ⋮ | ⋮ | ⋮ | ⋮ | ⋮ |
| 10 | 4.60 | 5.75 | 3.45 | 2.30 | 4.60 | 4.60 | 5.75 | 3.45 | 1.15 | 1.15 | 1.15 | 1.15 |
